# Supplementary material for: Towards Context-Aware Neural Performance-Score Synchronisation
Source: arXiv:2206.00454 source file (2022-05-31)
Supplement: Supplementary file 1 [file appendix.tex]

This section contains papers published / accepted for publication as part of this PhD. Following are the details of the papers:
\begin{itemize}
    \item A Hybrid Approach to Audio-to-Score Alignment: Published at International Conference on Machine Learning (ICML 2019) in the Machine Learning for Music Discovery Workshop
    \item Learning Frame Similarity using Siamese networks for Audio-to-Score Alignment: Accepted for publication at EUSIPCO 2020 (to be held in January 2021)
\end{itemize}
\includepdf[pages={1-4}]{icml2019_fixedTitle.pdf}
\includepdf[pages={1-5}]{EUSIPCO2020.pdf}
